# Supplementary material for: Benchmarking the ability of a controller to execute quantum error corrected non-Clifford circuits
Source: arXiv:2311.07121 source file (2025-08-29)
Supplement: Supplementary file 1 [file SM.pdf]

# Benchmarking the ability of a quantum controller to execute error corrected computation

# Supplementary materials

Yaniv Kurman[1], Lior Ella[1], Ramon Szmuk[1], Oded Wertheim[1], Benedikt Dorschner[2], Sam Stanwyck[2], and Yonatan Cohen[1]

[1]*Quantum Machines Inc., Tel Aviv, Israel*

[2]*NVIDIA Corp, Santa Clara, CA, USA*

### *S1 - The necessity of a feed-forward correction of a Pauli frame flip*

We present here a short example that shows a case where a Pauli frame flip propagates to a non-Clifford flip after two non-Cifford gates. Without the loss of generality, let us consider the following example, where we want to execute two non-commuting non-Clifford gates: $T = diag(1, e^{i\pi/4})$ followed by $X^{1/4}$ (as in Figure 3a in the main text), where the qubit experiences a Pauli $X$ error before the $T$ gate. After the $T$ gate, the $X$ frame is converted to a Clifford correction in the form of $TXT^{\dagger} = (X + Y)/\sqrt{2}$. Then, after the $X^{1/4}$ gate, the correction is converted to a non-Clifford gate (a $\pi$ rotation around the vector $(\frac{1}{\sqrt{2}}, \frac{1}{2}, \frac{1}{2})$) which cannot propagate efficiently in software throughout the quantum circuit. Therefore, from this example, we can deduce that a detection of a Pauli frame changes must be corrected through a circuit modification (or an active pulse) before the Pauli correction becomes a non-Clifford correction. Specifically, if the error is detected during the decoding of the $T$ gate, it should be corrected before the execution of the $X^{1/4}$ gate.

***S2 - How additional ancilla surfaces can ease the latency requirements***

As we explain in section III of the main text, and in section S1, fault-tolerant useful quantum calculations require feedback where the feed-forward type can change according to the specific non-Clifford gate (as in Figure 1b in the main text). However, there is a scheme, namely the auto-corrected $\pi/8$ scheme [S1], where the feed-forward logical gate remains independent of the executed non-Clifford gate. Moreover, this scheme can scale and ease the latency requirements with enough ancillary surfaces. The scheme can execute any Pauli (and multi-qubit Pauli) $\pi/8$ gate, as shown in Figure S1 for a single $T$ gate followed by a $X^{1/4}$ gate with two ancillary logical qubits for each non-Clifford gate.

Conceptually, the CDUs role does not change compared to the example in Fig 1 of the main text when executing a non-Clifford gate fault-tolerantly. That is, the execution of a planned gate includes an ancillary surface initialization stage, a lattice surgery stage, a logical measurement stage, and a feed-forward. The lattice surgery is performed between the surface that is initialized in the $|T\rangle = |0\rangle + e^{i\pi/4}|1\rangle$ state, the computational logical qubit (or qubits), and the $|0\rangle$ ancillary surface, producing two measurement results $m_0$ and $m_1$. As in the example in the main text, it is only the outcome from the surgery with the magic state ($m_1$) that determines the feed-forward conditional operation that will be in the form of the measurement basis of the second ancillary surface, i.e., whether to apply a Hadamard gate to the data qubits of this surface just before they are measured. To successfully execute the planned non-Clifford gate, along with the subsequent non-Clifford gates, all four measurements, including those of the two ancilla surfaces, are required to determine the Pauli frame update for the computational surfaces.

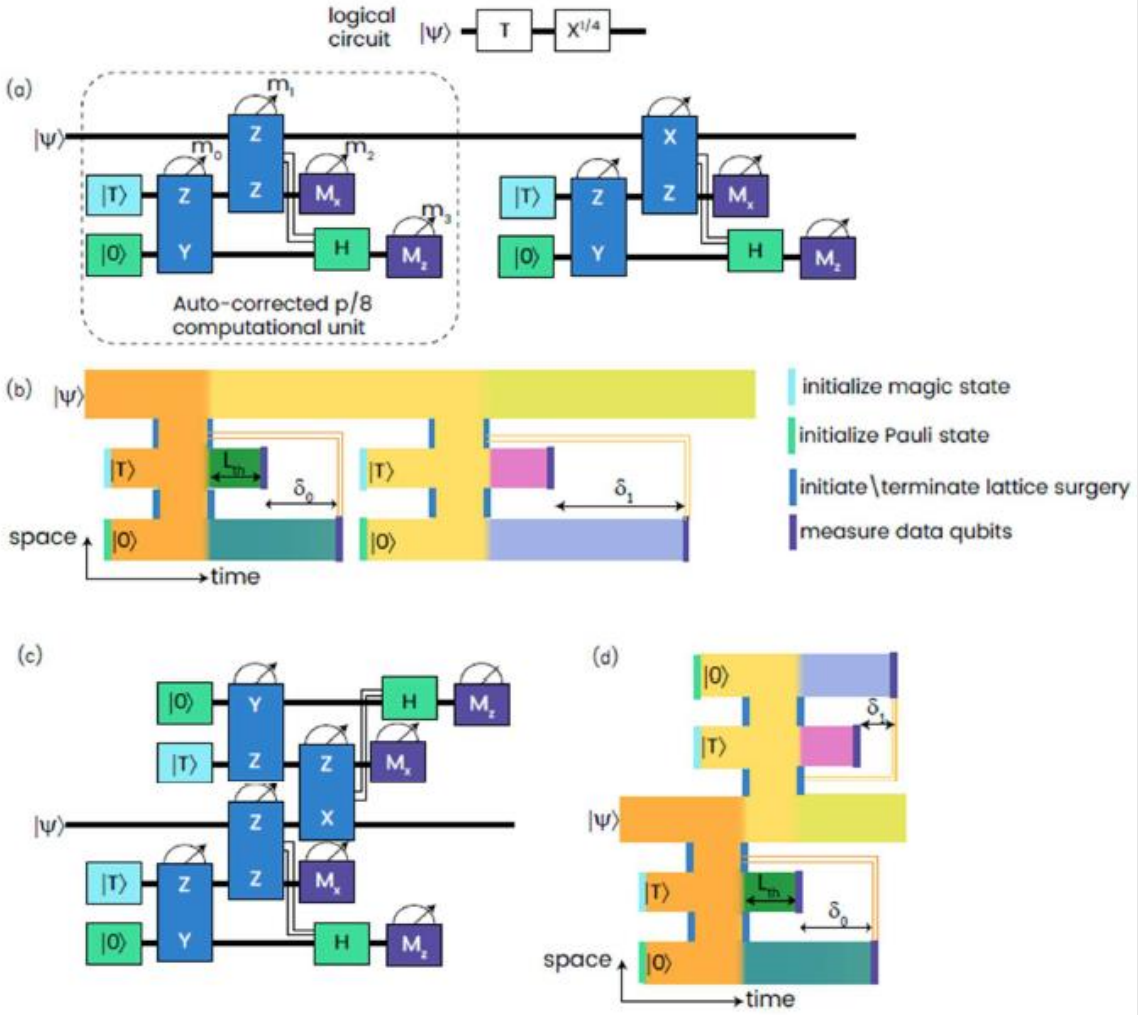


**Figure S1. Performing non-Clifford gates with the auto-corrected $\pi/8$ scheme. (a)** An example of the auto-corrected $\pi/8$ for performing a single $T$ gate followed by a $X^{1/4}$ gate with 2 ancilla surfaces. The scheme includes three stages (ancilla initialization, cyan; lattice surgery, blue; and measurement, purple), where the classical outcome of one of the surgeries ($m_1$) will determine the feed-forward in the form of a logical Hadamard gate to the second ancillary surface just before it is measured. Therefore, the second ancillary surface exhibits stabilizer rounds until the surgery decoding ends. This feed-forward (and also state initialization) is similar to every $\pi/8$ gate. **(b)** The surface view of the circuit in (a), with different decoding tasks in different colors. The threshold latency $L_{th}$ is determined by the number of rounds needed for a fault-tolerant logical measurement. **(c)** An implementation of a similar logical circuit with four ancillary surfaces. The additional surfaces eliminate any gap between the two non-Clifford gates, since the feed-forward is directed to an ancillary surface rather than the computational one. **(d)** The surface view of the circuit in (c), showing how four ancilla surfaces reduce the computation time. Through this view, it becomes evident that another contribution to the reduction in computation time is achieved by decreasing the data analyzed by the decoder (yellow decoding task), thereby reducing the circuit delay ($\delta_1$).

The auto-corrected $\pi/8$ scheme has additional advantages when allowing more than two ancillary surfaces. For example, when having four ancillary surfaces (as shown in Figure S1c), the additional surfaces enable performing two non-Clifford gates without any gaps in time between the gates. This is enabled because the feed-forward is applied to an ancillary surface rather than the computational surface. This capability yields another advantage: as the computational surfaces don't require waiting, the decoder processes a reduced number of syndromes (depicted in yellow area in Figure S1d compared to yellow area in S1b), resulting in an overall reduced feed-forward latency (FFL). Therefore, not only the second non-Clifford gate can start before the feed-forward of the first non-Clifford gate is applied, the additional ancillary surfaces enable a smaller latency, and thus a reduced logical clock. A similar effect will happen when six ancillary surfaces are available (Figure S2a), where the difference compared to four surfaces is that three consecutive nonstop non-Clifford gates can be applied (and further nonstop gates if $L < L_{th}$). Only when the number of ancillary surfaces increases to eight (Figure S2b), $L_{th}$ starts to increase without increasing the decoding task area. Figure S3 presents the effect of increasing the threshold latency on the decoding latencies for various classical configurations. As $L_{th}$ increases, the requirements on the classical computation are relieved.

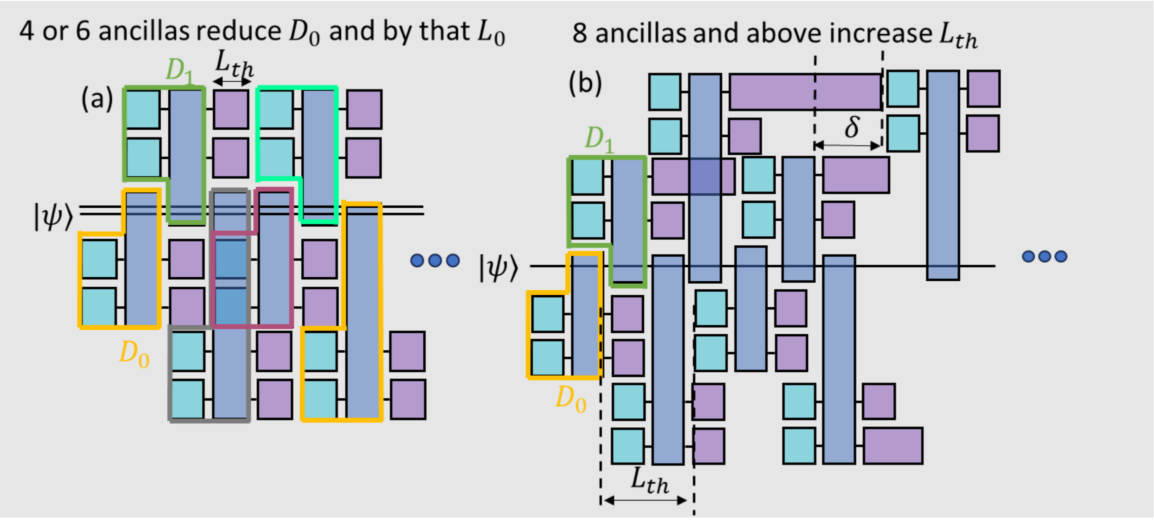


**Figure S2. The $\pi/8$ architecture for 6 (a) and 8 (b) ancilla surfaces.** In both panels, the computational surfaces ($|\psi\rangle$) are continuously involved in a lattice surgery, i.e., without any stabilizer rounds where the computational surfaces are not involved in lattice surgery. Each main decoding task is encircled in a different color. Since there are three basic operations (surface initialization, lattice surgery, and logical measurement) at least eight ancillary surfaces are needed to increase $L_{th}$.

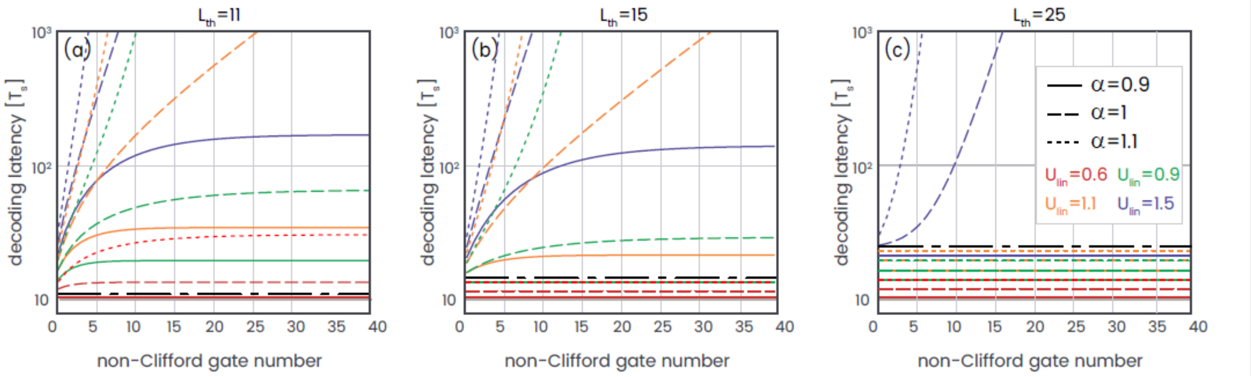


**Figure S3: The effect of the threshold latency on the decoding latency.** The decoding latency for different threshold latencies and classical parameters (denoted in panel (c)). If $L_{th}$ is increased beyond $L^0$, fault-tolerant quantum computation can be executed even when using a seemingly impractical classical decoder (large linear utilization $U_{lin}$ and complexity $\alpha$).

## *S3 - Analysis of the linear decoder behavior*

In this analysis we address the case where the FFL grows linearly with the number of data it receives, $L(N) = \tau_0 + N/T$, with $\tau_0$ being a latency offset and $T$ is the decoder's throughput. As we explained in the main text, if there is a round where $L^{(n)} > L_{th}$ (for simplicity let's denote the latency of this round as $L_0$), then the additional data in the following decoding task becomes $N^{(1)}(L_0) = N_0 + \lambda(L_0 - L_{th})$. We note that the for surface code architecture, the syndrome arrival rate to the decoder can be expressed as $\lambda = \frac{pM_c d^2}{T_s}$ where $M_c$ is the number of computational surfaces, $d$ is the code distance, $T_s$ is the time of a stabilizer rounds, and $p$ is the probability that a measurement is a syndrome defect. Thus, the additional data of $N^{(1)}$ compared to $\mathrm{N}_0$ arises from stabilizer rounds of the computational surfaces that wait for the next lattice surgery. Due to this additional data, the consequent FFL becomes

$$L^{(1)} = \tau_0 + \frac{\mathrm{N}^{(1)}}{T} = \tau_0 + \frac{N_0 + \lambda(L_0 - L_{th})}{T} = L^0 + \frac{\lambda}{T}(L_0 - L_{th}) = L_0 + U(L_0 - L_{th}) \quad (S1)$$

where $U$ is the utilization of the decoder. Similarly, the latency of the next non-Clifford gate will be

$$L^{(2)} = L_0 + U(L^{(1)} - L_{th}) = L^{(1)} + U^2(L_0 - L_{th}) = L_0 + U(U+1)(L_0 - L_{th}),$$

which we can continue recursively to the latency of the $n$'th non-Clifford gate,

$$L^{(n)} = L^{(n-1)} + U^n(L_0 - L_{th}) = L_0 + (L_0 - L_{th})\sum_{k=1}^{n} U^k = L_0 + (L_0 - L_{th})\frac{U(U^n - 1)}{U - 1}. \quad (S2)$$

From Eq. (S2) we can see that the latency diverges with $n$ if the decoder's utilization satisfies $U > 1$. This condition will occur if syndrome generation rate is larger than the decoder's throughput.

```
func initialize_surface(logical_qubit, state):
        active_logical_qubits.append(logical_qubit)
        for data_qubit in logical_qubit.data_qubits:
                reset(data_qubit)
                if state:
                        play(pi,data_qubit)

func play_x(logical_qubit):
        for data_qubit in logical_qubit.data_qubits:
                play(pi,data_qubit)

func measure_surface(logical_qubit,error_probability):
        active_logical_qubits - = logical_qubit
        return measure_qubits(logical_qubit.data_qubit_resonators, error_probability)

func stabilizer_round(error_probability, round_time):
        for logical_qubit in active_logical_qubits:
                ancilla_bits=measure_qubits(logical_qubit.ancilla_qubit_resonators,
error_probability)
        wait_until(round_time)
        return ancilla_bits

func measure_qubits(qubit_resonators, error_probability):
        discr_threshold=threshold(error_probability)
        for i, resonator in enumerate(qubit_resonators):
                measure(readout_pulse, resonator, demod(x))
                state[i] = x > discr_threshold
        return state

func initialize_surgery(logical_qubit1,logical_qubit2):
        active_logical_qubits - = logical_qubit1
        active_logical_qubits - = logical_qubit2
        active_logical_qubits.append(logical_qubit1+logical_qubit2+sugregy_qubits)
        for data_qubits in sugregy_qubits.data_qubits:
                reset(data_qubit)

func terminate_surgery((logical_qubit1,logical_qubit2),error_probability)
        measure_qubits(sugregy_qubits.data_qubits, error_probability))
        active_logical_qubits - =(logical_qubit1+logical_qubit2+sugregy_qubits)
        active_logical_qubits.append(logical_qubit1)
        active_logical_qubits.append(logical_qubit2)
```

**Listing S1: Pseudocode for the macros in the benchmark definitions.** Color coding is the same as in Listing 1 in the main text. The parameter **discr_threshold** is the discrimination threshold, chosen such that white noise in the analog channels will have a probability according to the **error_probability** that can probabilistically create an error for a specific qubit resonator, given the measurement history (denoted by **meas_history** which includes all measurement results so far) to be above it. We define the benchmarks for a 7-to-1 readout multiplexing so that a Surface-49 will have 7 pairs of analog channels for all measurements. We note also that the command **reset** can be defined as a macro with iterations in quantum-real-time to reach a high fidelity.

**Table S1: Simulation parameters of Figure 4 in the main text**

<table>
<tr><th>Figure</th><th>4a (purple)</th><th>4b</th><th>4c</th><th>4d</th><th>S3</th></tr>
<tr><td>code distance d</td><td colspan="5">5</td></tr>
<tr><td>syndrome probability $p$</td><td colspan="5">0.01</td></tr>
<tr><td># computational surfaces $M_c$</td><td colspan="5">2</td></tr>
<tr><td>number of initial syndromes $N_0$</td><td colspan="5">$3pM_cd^3$</td></tr>
<tr><td>latency offset coefficient $\tau_0$</td><td></td><td colspan="4">3</td></tr>
<tr><td>latency linear unitization $U_{lin}$</td><td></td><td colspan="3">variable</td><td>[0.6, 0.9, 1.1, 1.5]</td></tr>
<tr><td>latency prefactor $\tau_1$</td><td></td><td colspan="4">$U_{lin}/pM_cd^2$</td></tr>
<tr><td>latency complexity factor $\alpha$</td><td></td><td colspan="2">variable</td><td>1</td><td>[0.9, 1, 1.1]</td></tr>
<tr><td>Initial latency $L^0$</td><td></td><td colspan="4">$\tau_0 + \tau_1(N_0)^\alpha$</td></tr>
<tr><td>threshold latency $L_{th}$</td><td colspan="4">11</td><td>[11, 15, 25]</td></tr>
</table>

**Table S2: Simulation parameters of Figure 5c in the main text.** The total latency, plotted in Fig. 5c is calculated as the sum of the latencies below, where the sub-optimal plots change one of the parameters of the state-of-the-art system. We combine the bandwidths of the controller and communication channel, as the latter is expected to be the limiting factor due to its lower degree of distribution. Similarly, we treat their latencies jointly, since the mapping from analog-to-digital conversion to a communication packet bit is inherently tied to the controller's architecture and cannot be decoupled. We note that $N$ corresponds to the number of syndromes to be decoded, taken as $N = 0.025d\frac{d^2-1}{2}$ for a physical error rate of 0.005 [S5].

| | State-of-the-art | Sub-optimal |
|---|---|---|
| **Controller and communication minimal latency (round-trip)** | 3.5 $\mu$s [S3, S4] | 10 $\mu s$ |
| **Controller and Communication Bandwidth**<br>Corresponding latency | 64 Gb/s [S3]<br>$\frac{d^2}{64}\ ns$ | 250 Mb/s<br>$4\ d^2\ ns$ |
| **Decoding latency** | Sub-linear<br>$15 + 160 \cdot N^{0.23}$ ns [S2] | Linear<br>2000+200$N$ ns |

## Supplementary references


[S1] Litinski, Daniel. "A game of surface codes: Large-scale quantum computing with lattice surgery." *Quantum* 3 (2019): 128.

[S2] Liyanage, Namitha, et al. "FPGA-based distributed union-find decoder for surface codes." *IEEE Transactions on Quantum Engineering* 5 (2024): 1-18.

[S3] Mohseni, Masoud, et al. "How to build a quantum supercomputer: Scaling challenges and opportunities." *TBD* FERMILAB-PUB-24-0843-ETD; arXiv: 2411.10406 (2024).

[S4] Caune, Laura, et al. "Demonstrating real-time and low-latency quantum error correction with superconducting qubits." *arXiv preprint arXiv:2410.05202* (2024).
